# Supplementary material for: MSI: Maximize Support-Set Information for Few-Shot Segmentation
Source: arXiv:2212.04673 source file (2023-11-10)
Supplement: Supplementary file 1 [file appendix.tex]

% \begin{center}
%  {\section*{Supplementary Materials for Paper ID 4759: MSI: Maximize Support-Set Information for Few-Shot Segmentation}}
% \end{center}
\begin{center}
 {\section*{Supplementary Materials}}
\end{center}

MSI shows that background information overlooked by existing methods can help to segment a target. By utilizing both STF and SIF, MSI is able to obtain information on the target class from the entire support image while minimizing bias to the target class. Through STF, MSI is able to obtain more fine-grained target information which potentially gets removed by masking background features. By using SIF, it becomes possible to acquire more information about the target that might have been missed by the limited support mask. Furthermore, it utilizes other objects in the background of the support image to either avoid segmenting non-target objects or aid segmenting the target object in the query image. In this supplementary material, we include the following items:

% \begin{enumerate}[topsep=-3pt, noitemsep]
\begin{enumerate}[label={A.}{{\arabic*}},noitemsep,itemindent=0.5cm]
\item Correlation map analysis.
\item Detailed architecture.
\item Training profiles.
\item Data augmentation.
\item Differences between VAT \& VAT~+~MSI.
\item Additional qualitative results.
\item Failure cases.
% \item Limitation and Future works.
\end{enumerate}

\subsection*{A.1~Correlation Map Analysis}
Since FM~(Feature Masking) eliminates background features, high correlation values exist only within the target object area~(Fig.~\ref{fig:correlation_compare}).
% When the support mask does not accurately cover the entire target object, this results in giving limited target information to a network~(see Fig.~\ref{fig:correlation_compare2}). 
When the support mask does not accurately cover the entire target object, the target information received by a network is limited~(Fig.~\ref{fig:correlation_compare2}). 

The support target features (STF) have high activation around the target object in the support image but not in the query image. Some background areas in the support image features (SIF) are activated because they match the background features of the query image. Although both SIF and STF weakly capture the target object of the query image in their correlation maps, once these correlation maps are fed to the encoder, in the encoded feature maps, we observe strong signals across the target class of the query image ~(see the feature map in Fig.~\ref{fig:correlation_compare}). On the contrary, the FM encoder produces a more scattered activation around the target.

% \replace{the features from the entire support image are matching to the background in}{they match the background features of} the query image.

% However, this is not an issue, because the background areas in the support image features (SIF) are highly correlated with the background of the query image.

% Although both SIF and STF weakly capture the target object of the query image in their correlation maps, once these correlation maps are fed to the encoder, in the encoded feature maps, we observe strong signals around the target class of the query image.
% Both SIF and STF weakly capture the target object of the query image in their correlation maps, because of the aforementioned relationship between their target and background features. However, the encoder is able to exploit these correlation maps to produce strong signals within and around the target class of the query image~(see the feature map in Fig.~\ref{fig:correlation_compare}).
% Whereas in FM the attention is much more scattered in the encoded feature maps.
% On the contrary, the FM encoder produces a more scattered activation around the target.

%loses attention bit to where to focus on.

% Fig.~\ref{fig:correlation_compare} shows which features are attracting attention through the correlation map when using the MSI method. MSI can confirm that all features are activated. And when this correlation map passes through the encoder, it can be confirmed that a strong signal is formed in the target object.

\subsection*{A.2~Detailed Architecture}
In Fig.~\ref{fig:overall} of the main manuscript, the encoder part is shown briefly. In Fig.~\ref{fig:detail_architecture}, we reveal more details relevant to the encoder that are specific to each baseline architecture: HSNet~\cite{HSNet}, VAT~\cite{VAT} and, ASNet~\cite{ASNet}. For HSNet, the SCM is divided into 3 convolutional blocks and used in 3 stages of the encoder step-by-step. VAT utilizes query features again in the decoding stage. ASNet uses pooling to reduce the input feature size.

%schematically expressed briefly but in detail, as shown in Fig.~\ref{fig:detail_architecture}, the SCM is divided into 3 conv blocks and used in 3 stages of the encoder step by step. HSNet~\cite{HSNet}, VAT~\cite{VAT2}, and ASNet~\cite{ASNet} used a similar approach but there are some variation. VAT utilized the query features in the decoder once again, and ASNet used pooling to reduce the input feature size.

\begin{figure}[h]
  \centering
    \includegraphics[height=6.0cm]{iccv/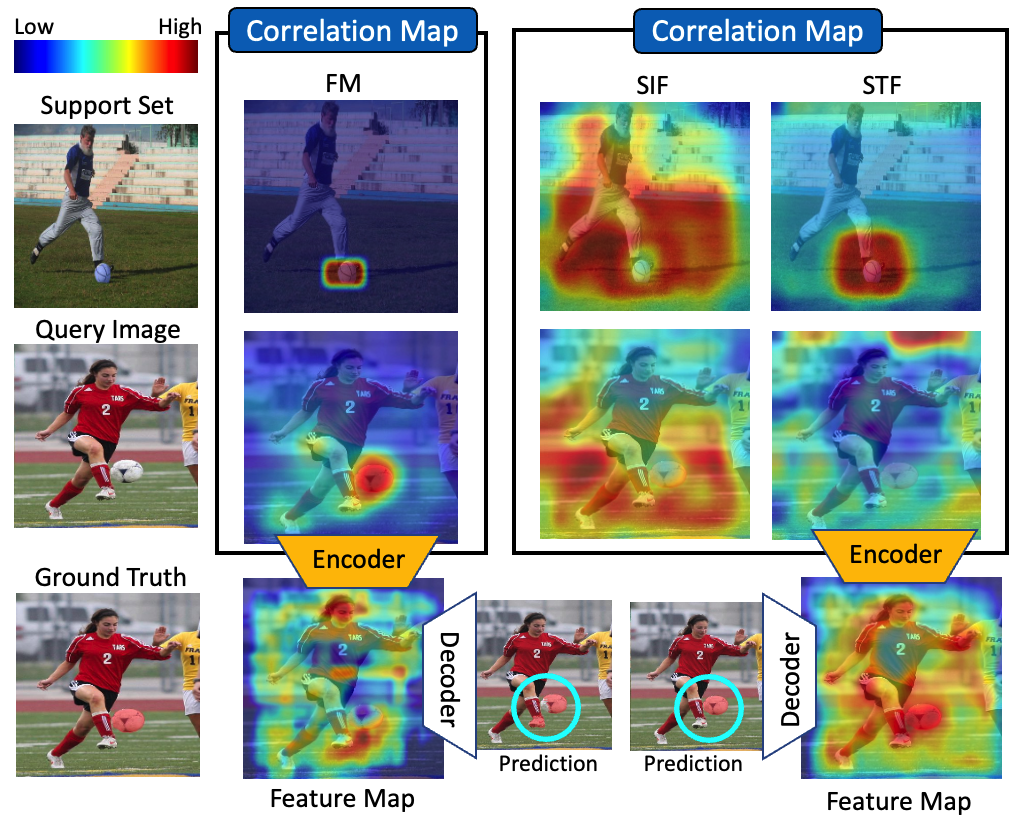}
    \caption{Correlation map and feature map visualization. Although STF and SIF weakly capture the target class of the query image in their correlation maps, once these correlation maps are fed to the encoder, we notice strong signals on the target object.}
    \label{fig:correlation_compare}
\end{figure}

\begin{figure}[h]
  \centering
    \includegraphics[height=7.8cm]{iccv/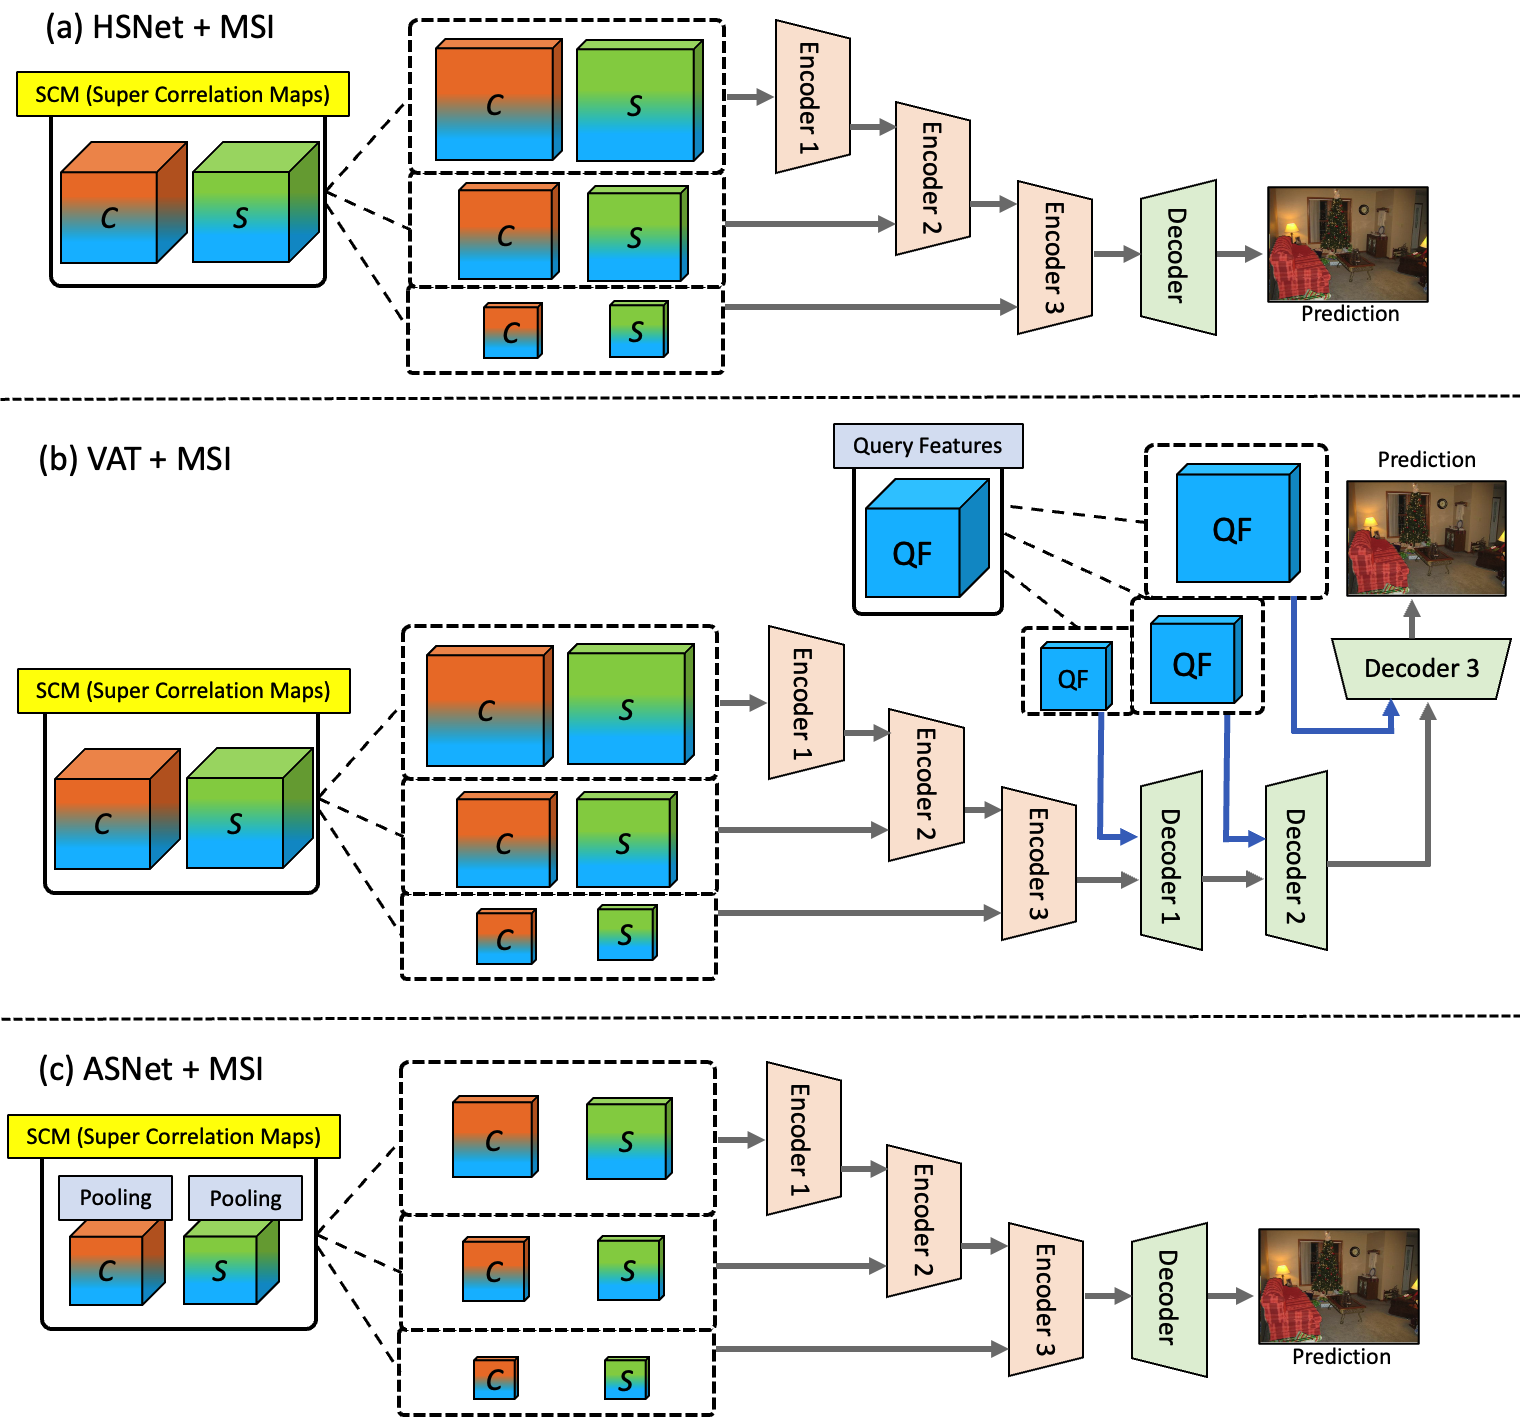}
    \caption{Detailed architectures showing where SCM is used for HSNet~\cite{HSNet}, VAT~\cite{VAT}, and ASNet~\cite{ASNet}. (a)~HSNet~+~MSI (b)~VAT~+~MSI (c)~ASNet~+~MSI.}
    \label{fig:detail_architecture}
\end{figure}

\subsection*{A.3~Training Profiles} Figure~\ref{fig:train_curve} (main paper) shows that VAT~+~MSI provides 3.5x faster convergence compared to VAT~\cite{VAT}. In Fig.~\ref{fig:train_curve_hsnet}, we reveal that our MSI with HSNet baseline, HSNet~+~MSI, enables 4.5x faster convergence in comparison to HSNet~\cite{HSNet}. This could be because STF provides a strong prior on the target boundary information to the encoder network. 

% signal of the edge of the target feature

% that the training speed improved rapidly as the strong signal of the edge of the target feature was given to the network by using STF.

% VAT~+~MSI improved the training speed by 3.5 times compared to VAT~\cite{VAT2},  

% HSNet~+~MSI showed the training speed was 4.5 times faster than HSNet~\cite{HSNet}~(see Fig.~\ref{fig:train_curve_hsnet}).

\begin{figure}[h]
  \centering
    \includegraphics[height=8.3cm]{iccv/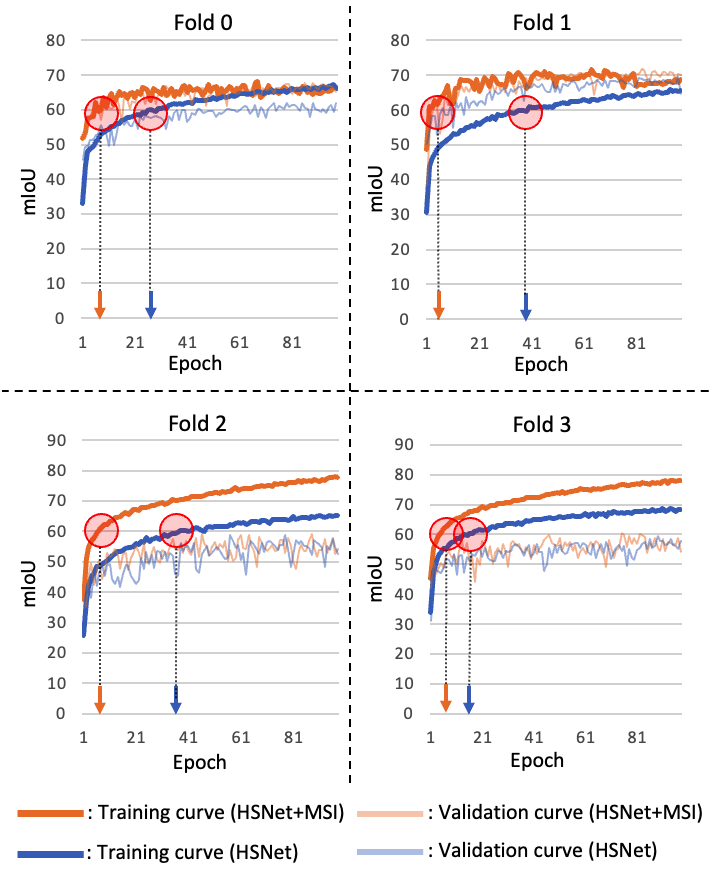}
    
   \caption{Train.~and~Val.~profiles of HSNet~\cite{HSNet} and HSNet+MSI on PASCAL-5$^i$~\cite{pascal} with ResNet50~\cite{Resnet}. HSNet+MSI provides 4.5x faster convergence (to reach 60\% in mIoU) on average than HSNet. Red circles indicate when train accuracy reaches 60\% in mIoU.}
   \label{fig:train_curve_hsnet}
\end{figure}

% it still has a lot of potential for improvement under following challenging conditions. 

% When only the small part of the target object in the support set is given, the target object could not be accurately segmented in the query image, and MSI did not show good performance when the image quality of the target object in the query image was poor. Also, when the color or shape of the target object was different, the performance improvement was minimal~(see Fig.~\ref{fig:pascal_fail} and Fig.~\ref{fig:coco_fail}).

\subsection*{A.4~Data Augmentation.}

% \begin{table}[h]
%   \centering
%     \begin{minipage}{.47\textwidth}
% \centering
% \resizebox{\textwidth}{!}{
% \begin{tabular}{@{}cc|ccccc}
% \toprule
% \multirow{2}{*}{Backbone} & \multirow{2}{*}{Methods} & \multicolumn{5}{c}{1-shot} 
% \\
%  &  & $20^0$ & $20^1$ & $20^2$ & $20^3$ & mIoU   \\ \midrule
% \multirow{4}{*}{ResNet50~\cite{Resnet}} 
% &VAT~\cite{VAT2} & 67.6 & 72.0 & 62.3 & 60.1 & 65.5  \\ 
% & VAT$^\ast~$~\cite{VAT} & {67.6} & {71.2} & {62.3} & {60.1} & {65.3} \\ 
% &VAT~+~MSI & 69.9 & 72.0 & 61.5 & 65.5 & 67.2  \\ 
% & VAT$^\ast~$+~MSI & \textbf{71.0} & \textbf{72.5} & \textbf{63.8} & \textbf{65.9} & \textbf{68.3} \\ 
% \midrule

% \multirow{4}{*}{ResNet101~\cite{Resnet}} 
% &VAT~\cite{VAT2} & 70.0 & 72.5 & 64.8 & 64.2 & 67.9 \\
% & VAT$^\ast~$~\cite{VAT} & {68.4} & {72.5} & {64.8} & {64.2} & {67.5} \\ 

% &VAT~+~MSI & 71.0 & 73.2 & \textbf{65.1} & 66.5 & 68.9 \\ 
% & VAT$^\ast~$+~MSI & \textbf{73.1} & \textbf{73.3} & {64.7} & \textbf{68.8} & \textbf{70.0} \\ 

% % 73.1 73.3 64.7 68.8 70.0

% \bottomrule 
% \end{tabular}

% }

%     \end{minipage}
%     \caption{The impact of data augmentation on VAT and VAT~+~MSI on PASCAL-5$^i$~\cite{pascal} dataset. $^\ast$~indicates that data augmentation is used for training. Best results are shown in \textbf{bold}.} 
    
% \label{table:data_augmentation}

%   \end{table}

\begin{table}[h]
\centering
\scalebox{0.7}{%
 \begin{tabular}{c | c c | c c} 
 \hline
 Method \& Backbone & Data Aug.  & MSI & mIoU & FB-IoU \\
 \hline
 & - & -  &  65.5 & 77.8 \\
VAT~\cite{VAT} & \checkmark & - & 65.3  &  77.4 \\ 
(ResNet50~\cite{Resnet}) & - & \checkmark  &  67.2 & 78.6 \\
 & \checkmark & \checkmark  &  \textbf{68.3} & \textbf{79.1} \\
\hline
 & - & -  &  67.9 & 79.6 \\
VAT~\cite{VAT} & \checkmark & -  & 67.5 & 78.8 \\ 
(ResNet101~\cite{Resnet}) & - & \checkmark  &  68.9 & 79.4 \\
 & \checkmark & \checkmark  &  \textbf{70.1} & \textbf{82.3} \\
\hline
 \end{tabular}
 }
\caption{The impact of data augmentation on VAT~\cite{VAT} and VAT~+~MSI on PASCAL-5$^i$~\cite{pascal}. Best results are shown in \textbf{bold}.} 
    
\label{table:data_augmentation}
\end{table}

VAT~\cite{VAT2} does not recommend using data augmentation~\cite{data_aug_1, data_gug_2} as it causes performance drop. However, when using our proposed method with VAT, the performance improves using CATs data augmentation~\cite{data_gug_2} (see Tab.~\ref{table:data_augmentation}). 

% As the STF provides strong target information to the network, training speed becomes very fast and over-fitting starts very early. To mitigate over-fitting, CATs data augmentation was useful.

%As the STF provides strong target information to the network, training speed becomes very fast and over-fitting starts very early. To mitigate over-fitting, CATs data augmentation was useful.

% , data augmentation~\cite{data_aug_1, data_gug_2, VAT} was not recommended to use because it tends to perform. However, when using our proposed method, VAT~+~MSI is trained stably and showed better performance than without using data augmentation (see Tab.~\ref{table:data_augmentation}). 

\subsection*{A.5~Differences between VAT \& VAT~+~MSI.}
VAT performs 
% complementary support
correlation mapping only between query features~(QF) and masked support features. We term the masked support features as feature masking~(FM) (Fig.~\ref{fig:4cases}). FM loses 
fine-grained target information such as textures and boundaries because of 
late-stage masking and masking features with inaccurate support masks~(Fig.~\ref{fig:feature_analysis}, Fig.~\ref{fig:receptive_field}), which limits VAT.
% masking features that could hold target information~(Fig. 8, Fig.~\ref{fig:receptive_field}) and masking features with inaccurate support mask (Fig.~1). 
% Therefore, 
% the performance of 
% VAT is limited by FM. 
% Unlike FM, MSI utilizes both masked image and entire image to extract support target features~(STF) and support image features~(SIF). STF, which has more fine detailed target information than FM, helps the network to activate target features while simultaneously deactivating background features in SIF.
VAT+MSI utilizes both SIF and STF (Fig.~\ref{fig:teaser}) to compute correlation maps $CS_1$ and $CS_2$ respectively with QF. $CS_1$ allows the network to learn additional contextual target information in SIF~(e.g., in the background), whereas $CS_2$ uses STF to mask the input and has
% more fine-detailed and
stronger target information than FM, which helps the network to activate target foreground features while simultaneously deactivating target-irrelevant background features in SIF.
This way, by maximizing target information, MSI can boost performance.

\subsection*{A.6~Additional Qualitative Results.}
Figs.~\ref{fig:pascal_msi}, \ref{fig:coco_msi}, and \ref{fig:fss_msi} show additional qualitative results of VAT~+~MSI on three benchmarks.

\subsection*{A.7~Failure Cases}
Although MSI shows significant gains over strong FSS baselines, we identify some challenging FSS cases where there is still room for improvement.
When a very small part of the target object in the support set is given, the target object might not be accurately segmented in the query image (see the fourth row in Fig.~\ref{fig:coco_fail}). Also, when the target object in the query image lies far in the background and appears blurry (see the fifth row in Fig.~\ref{fig:pascal_fail}), the segmentation accuracy could worsen.
Other challenging cases are when the color or shape of the target object is quite different ~(see the third row in Fig.~\ref{fig:pascal_fail} and the third row in Fig.~\ref{fig:coco_fail}) and when the object class in the support set and query image are not the same, but are similar in shape and semantics, such as a computer monitor vs. television (see the second row in Fig.~\ref{fig:pascal_fail}). 

% (see the second row in Fig.~\ref{fig:pascal_fail}); rather they are neighbors (PC monitor vs. television or LCD vs. CRT legacy tube screen
% two objects do not belong to the same class (see the second row in Fig.~\ref{fig:pascal_fail}); rather they are neighbors (PC monitor vs. television or LCD vs. CRT legacy tube screen)

\begin{figure}[h]
  \centering
    \includegraphics[height=13.1cm]{iccv/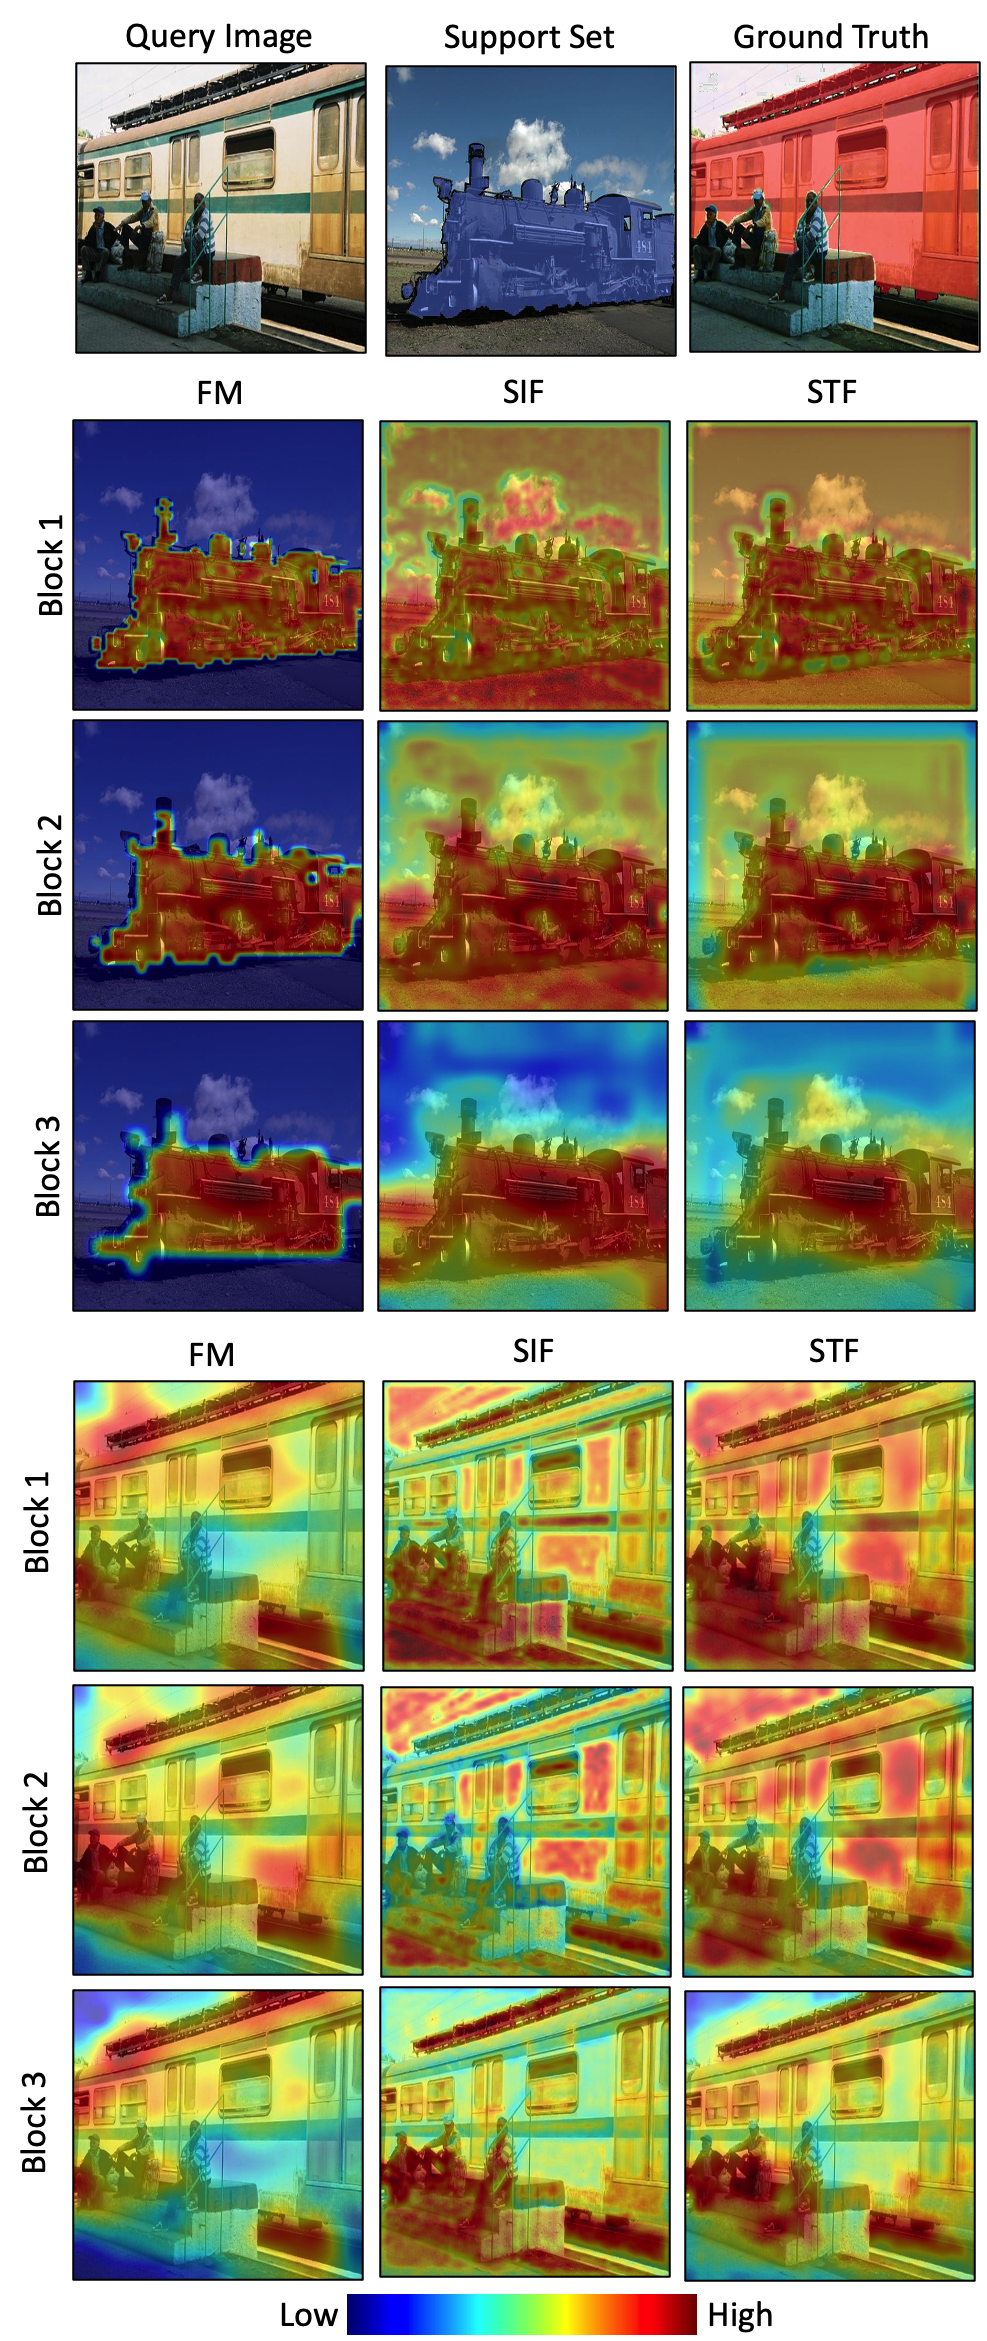}
    \caption{Correlation map visualization. Feature masking~(FM) with the inaccurate support mask causes inadvertent loss in the boundary information of the target. On the other hand, Support Image Features~(SIF) utilizes the entire image features and the Support Target Features~(STF) focuses on the target after removing the background at the input level. Note that in the Block 1, compared to FM, STF has distinct signals at the target class boundary. In the Block 3, compared to FM, in SIF, the correlation is evenly distributed across various areas in the target object.}
    \label{fig:correlation_compare2}
\end{figure}

% By giving meaningful target information with STF, rather than picking up noise in the input data through data augmentation to confuse the network, it shows that it is useful for learning more diverse input data and shows a robust training network.

% \subsection*{A.6~Limitation and Future works}

\begin{figure}
  \centering
    \includegraphics[height=21.4cm]{iccv/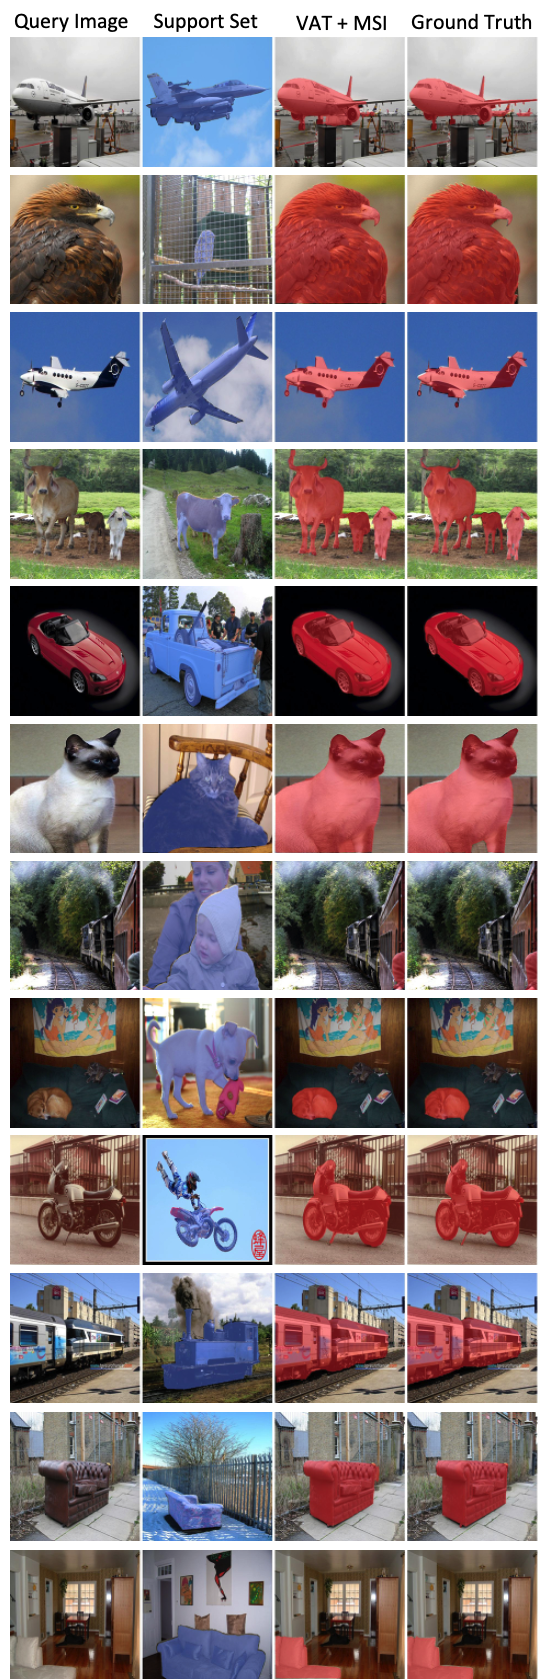}
    \caption{VAT~+~MSI Qualitative result using ResNet50~\cite{Resnet} on PASCAL-5$^i$~\cite{pascal}.}   \label{fig:pascal_msi}
\end{figure}

\begin{figure}
  \centering
    \includegraphics[height=21.4cm]{iccv/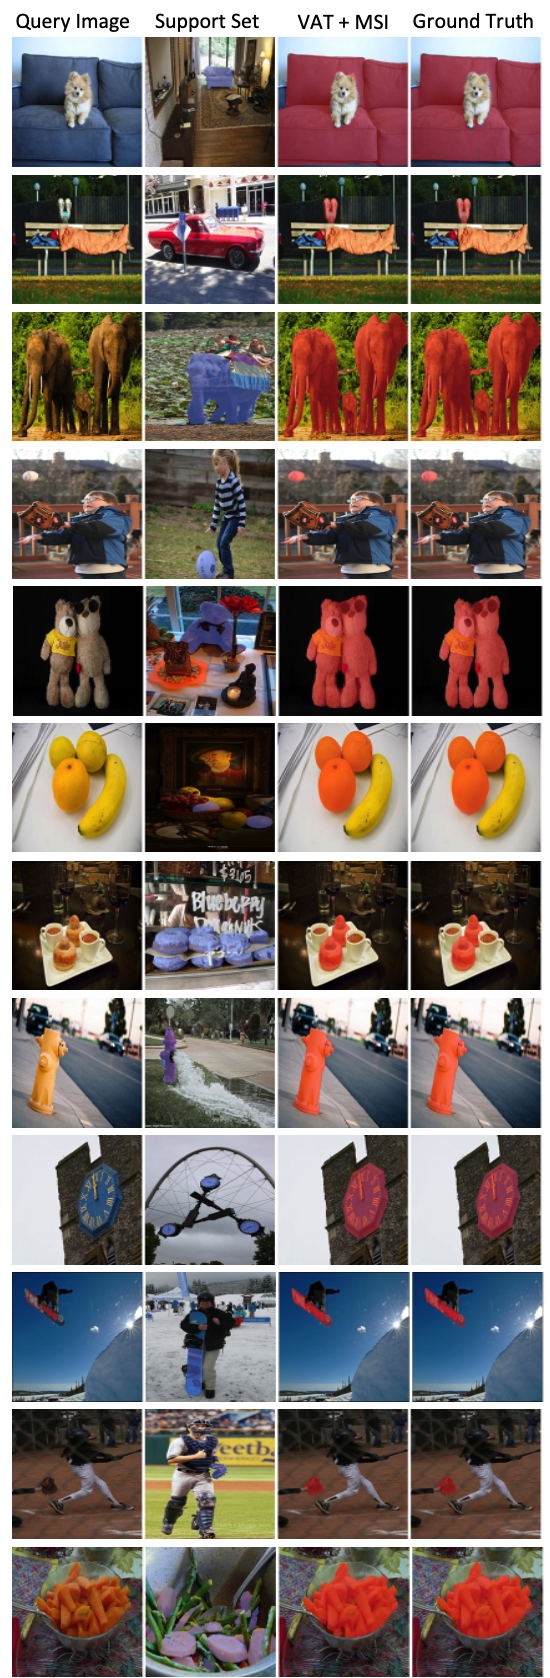}
    \caption{VAT~+~MSI Qualitative result using ResNet50~\cite{Resnet} on COCO-20$^i$~\cite{lin2015microsoft}.}    \label{fig:coco_msi}
\end{figure}

\begin{figure}
  \centering
    \includegraphics[height=21.4cm]{iccv/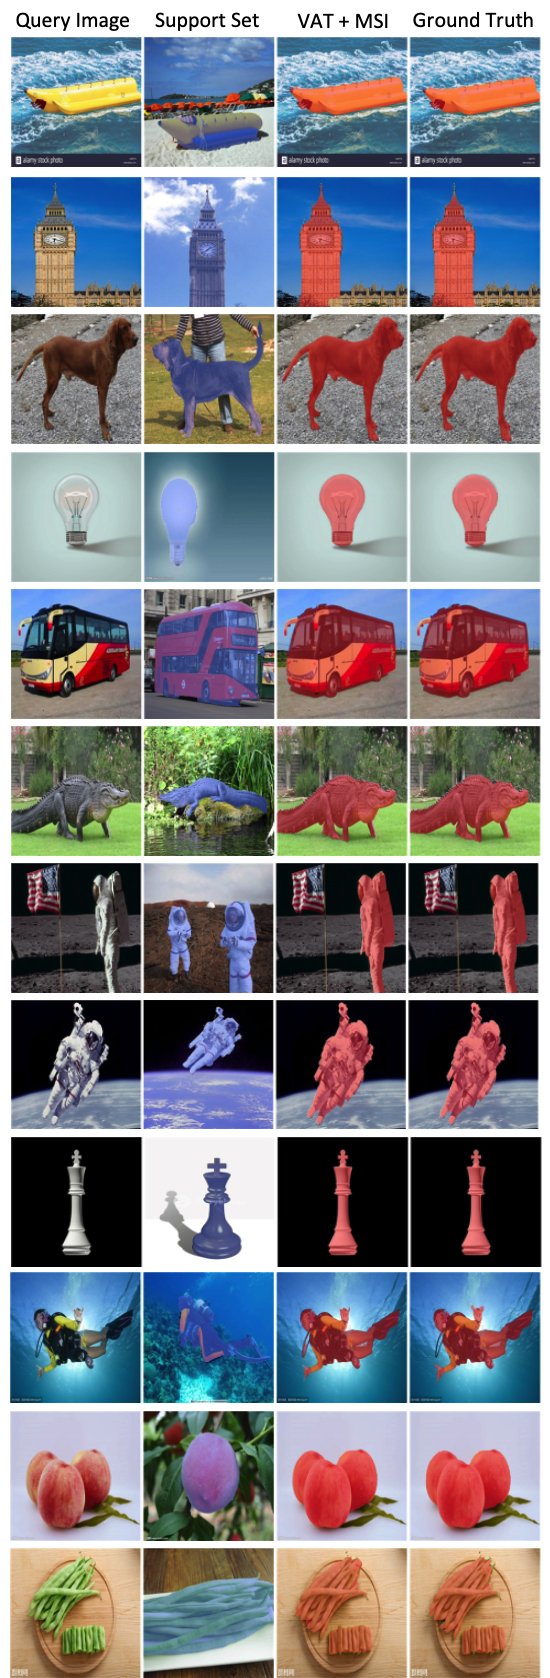}
    \caption{VAT~+~MSI Qualitative result using ResNet50~\cite{Resnet} on FSS-1000~\cite{FSS1000}.}
    \label{fig:fss_msi}
\end{figure}

\begin{figure}
  \centering
    \includegraphics[height=8.6cm]{iccv/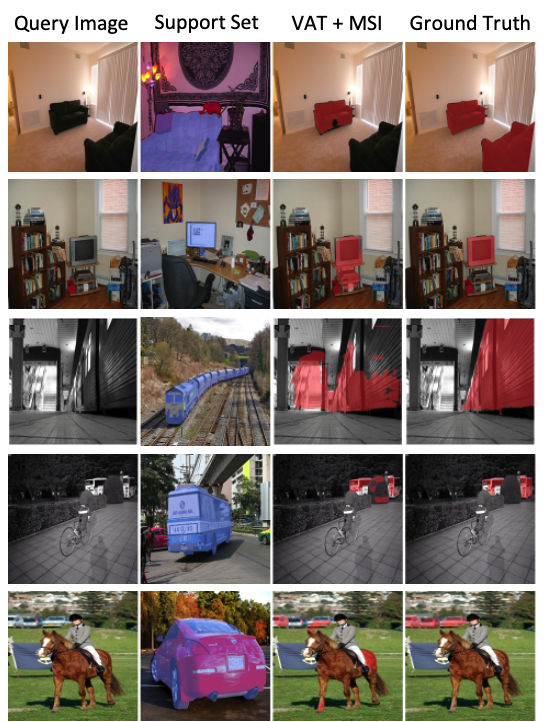}
    \caption{Failure cases of VAT~+~MSI with ResNet50~\cite{Resnet} on PASCAL-5$^i$~\cite{pascal}.}
    \label{fig:pascal_fail}
\end{figure}

\begin{figure}
  \centering
    \includegraphics[height=8.6cm]{iccv/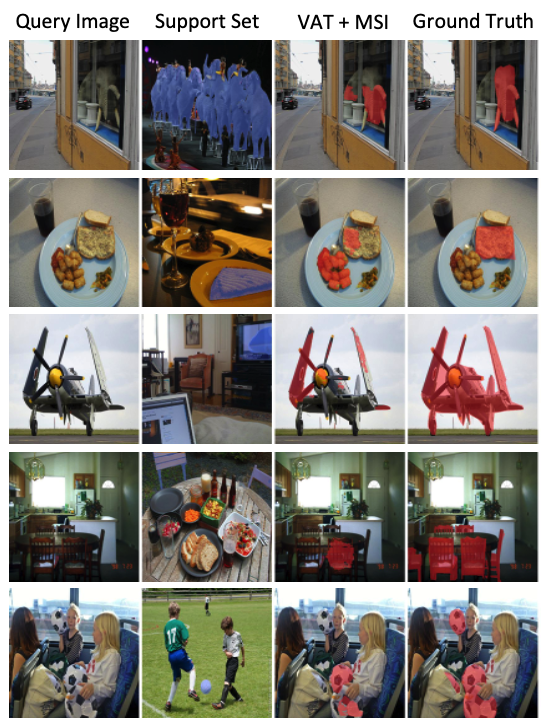}
    \caption{Failure cases of VAT~+~MSI with ResNet50~\cite{Resnet} on COCO-20$^i$~\cite{lin2015microsoft}.}
    \label{fig:coco_fail}
\end{figure}

% 1. Training profile figure (COCO, FSS with HSNet, VAT)

% 2. attention based merge architecture

% 3. more visual comparison figures

% 4. failure cases sutdy

% 5. Data augmentation explanation
